# Supplementary material for: A van der Waals density functional for solids
Source: arXiv:1209.3038 source file (2012-09-13)
Supplement: Supplementary file 1 [file supplemental_material.pdf]

# Supplemental material for "A van der Waals density functional for solids and surfaces"

Torbjörn Björkman

August 20, 2012

Table 1: AM05 binding energies for 26 layered solids. Energies are given in meV/Å$^2$. Compounds that has a local minimum near the experimental $c$ axis length have their binding energy marked with an asterisk (0*).

| Compound | $E_B$ | $E_B^{RPA}$ | RE [%] |
|---|---|---|---|
| BN | 0 | 14.49 | -100 |
| $HfS_2$ | 0 | 16.13 | -100 |
| $HfSe_2$ | 0 | 17.09 | -100 |
| $HfTe_2$ | 0.92 | 18.68 | -95.1 |
| $MoS_2$ | 0 | 20.53 | -100 |
| $MoSe_2$ | 0 | 19.63 | -100 |
| $MoTe_2$ | 0* | 20.80 | -100 |
| $NbSe_2$ | 0.42 | 19.57 | -97.9 |
| $NbTe_2$ | 3.05 | 23.03 | -86.7 |
| PbO | 1.66 | 20.25 | -91.8 |
| $PdTe_2$ | 24.1 | 40.17 | -40.0 |
| $PtS_2$ | 0 | 20.55 | -100 |
| $PtSe_2$ | 0* | 19.05 | -100 |
| $TaS_2$ | 0 | 17.68 | -100 |
| $TaSe_2$ | 0* | 19.44 | -100 |
| $TiS_2$ | 0 | 18.88 | -100 |
| $TiSe_2$ | 0* | 17.39 | -100 |
| $TiTe_2$ | 4.68 | 19.76 | -76.3 |
| $VS_2$ | 0* | 25.61 | -100 |
| $VSe_2$ | 0* | 22.26 | -100 |
| $WS_2$ | 0 | 20.24 | -100 |
| $WSe_2$ | 0 | 19.98 | -100 |
| $ZrS_2$ | 0 | 16.98 | -100 |
| $ZrSe_2$ | 0* | 18.53 | -100 |
| $ZrTe_2$ | 3.25 | 16.34 | -80.1 |
| Graphite | 0 | 18.32 | -100 |
| MRE | | | -94.9 |
| MARE | | | 94.9 |

Table 2: PW86R binding energies for 26 layered solids. Energies are given in meV/Å$^2$.

| Compound | $E_B$ | $E_B^{RPA}$ | RE [%] |
|---|---|---|---|
| BN | 0.36 | 14.49 | -97.5 |
| $HfS_2$ | 0.69 | 16.13 | -95.6 |
| $HfSe_2$ | 0.97 | 17.09 | -94.3 |
| $HfTe_2$ | 2.29 | 18.68 | -87.6 |
| $MoS_2$ | 0.64 | 20.53 | -96.8 |
| $MoSe_2$ | 0.60 | 19.63 | -96.9 |
| $MoTe_2$ | 1.59 | 20.80 | -92.3 |
| $NbSe_2$ | 1.99 | 19.57 | -89.7 |
| $NbTe_2$ | 1.82 | 23.03 | -92.0 |
| PbO | 3.39 | 20.25 | -83.2 |
| $PdTe_2$ | 10.30 | 40.17 | -74.3 |
| $PtS_2$ | 0.69 | 20.55 | -96.6 |
| $PtSe_2$ | 1.04 | 19.05 | -94.5 |
| $TaS_2$ | 1.36 | 17.68 | -92.2 |
| $TaSe_2$ | 2.23 | 19.44 | -88.4 |
| $TiS_2$ | 1.31 | 18.88 | -93.0 |
| $TiSe_2$ | 1.43 | 17.39 | -91.7 |
| $TiTe_2$ | 2.47 | 19.76 | -87.4 |
| $VS_2$ | 1.57 | 25.61 | -93.8 |
| $VSe_2$ | 1.61 | 22.26 | -92.7 |
| $WS_2$ | 0.55 | 20.24 | -97.2 |
| $WSe_2$ | 0.53 | 19.98 | -97.3 |
| $ZrS_2$ | 0.89 | 16.98 | -94.7 |
| $ZrSe_2$ | 1.30 | 18.53 | -92.9 |
| $ZrTe_2$ | 2.95 | 16.34 | -81.9 |
| Graphite | 0 | 18.32 | -100 |
| MRE | | -91.8 | |
| MARE | | 91.8 | |

Table 3: PBEsol binding energies for 26 layered solids. Energies are given in meV/Å$^2$.

| Compound | $E_B$ | $E_B^{RPA}$ | RE [%] |
|---|---|---|---|
| BN | 2.0 | 14.49 | -86.3 |
| $HfS_2$ | 3.0 | 16.13 | -81.4 |
| $HfSe_2$ | 4.3 | 17.09 | -74.7 |
| $HfTe_2$ | 9.5 | 18.68 | -49.0 |
| $MoS_2$ | 3.5 | 20.53 | -82.7 |
| $MoSe_2$ | 4.6 | 19.63 | -76.2 |
| $MoTe_2$ | 8.0 | 20.80 | -61.2 |
| $NbSe_2$ | 10.0 | 19.57 | -48.4 |
| $NbTe_2$ | 12.8 | 23.03 | -43.9 |
| PbO | 9.9 | 20.25 | -51.0 |
| $PdTe_2$ | 36.0 | 40.17 | -10.1 |
| $PtS_2$ | 5.5 | 20.55 | -72.7 |
| $PtSe_2$ | 10.7 | 19.05 | -43.6 |
| $TaS_2$ | 5.1 | 17.68 | -70.6 |
| $TaSe_2$ | 7.6 | 19.44 | -60.8 |
| $TiS_2$ | 6.5 | 18.88 | -65.3 |
| $TiSe_2$ | 8.7 | 17.39 | -49.5 |
| $TiTe_2$ | 14.4 | 19.76 | -26.7 |
| $VS_2$ | 7.6 | 25.61 | -70.0 |
| $VSe_2$ | 8.4 | 22.26 | -62.0 |
| $WS_2$ | 3.1 | 20.24 | -84.5 |
| $WSe_2$ | 4.2 | 19.98 | -78.8 |
| $ZrS_2$ | 3.6 | 16.98 | -78.3 |
| $ZrSe_2$ | 5.5 | 18.53 | -69.9 |
| $ZrTe_2$ | 12.4 | 16.34 | -24.0 |
| Graphite | 1.2 | 18.32 | -93.1 |
| MRE | | | -62.1 |
| MARE | | | 62.1 |

Table 4: PW86R-VV10 binding energies and relaxed geometries for 26 weakly bonded layered compounds. Energies are given in meV/Å$^2$ and lattice constants in Å.

| Compound | $E_B$ | $E_B^{RPA}$ | RE [%] | $c$ | $c^{exp}$ | RE [%] | $a$ | $a^{exp}$ | RE [%] |
|---|---|---|---|---|---|---|---|---|---|
| BN | 25.56 | 14.49 | 76.4 | 6.570 | 6.690 | -1.8 | 2.517 | 2.510 | 0.3 |
| $HfS_2$ | 24.67 | 16.13 | 52.9 | 5.811 | 5.837 | -0.5 | 3.673 | 3.635 | 1.0 |
| $HfSe_2$ | 25.36 | 17.09 | 48.4 | 6.192 | 6.159 | 0.5 | 3.800 | 3.748 | 1.4 |
| $HfTe_2$ | 27.69 | 18.68 | 48.2 | 6.749 | 6.650 | 1.5 | 4.016 | 3.957 | 1.5 |
| $MoS_2$ | 30.84 | 20.53 | 50.2 | 12.336 | 12.302 | 0.3 | 3.227 | 3.162 | 2.0 |
| $MoSe_2$ | 29.98 | 19.63 | 52.7 | 12.795 | 12.927 | -1.0 | 3.348 | 3.289 | 1.8 |
| $MoTe_2$ | 30.13 | 20.80 | 44.9 | 14.212 | 13.973 | 1.7 | 3.609 | 3.518 | 2.6 |
| $NbSe_2$ | 33.16 | 19.57 | 69.4 | 12.657 | 12.547 | 0.9 | 3.523 | 3.442 | 2.3 |
| $NbTe_2$ | 35.07 | 23.03 | 52.3 | 6.906 | 6.610 | 4.5 | 3.753 | 3.680 | 2.0 |
| PbO | 27.56 | 20.25 | 36.1 | 5.008 | 4.995 | 0.2 | 4.076 | 3.964 | 2.8 |
| $PdTe_2$ | 44.30 | 40.17 | 10.3 | 5.284 | 5.113 | 3.3 | 4.148 | 4.024 | 3.1 |
| $PtS_2$ | 31.67 | 20.55 | 54.1 | 4.975 | 5.043 | -1.4 | 3.642 | 3.542 | 2.8 |
| $PtSe_2$ | 30.43 | 19.05 | 59.8 | 5.123 | 5.081 | 0.8 | 3.846 | 3.727 | 3.2 |
| $TaS_2$ | 31.38 | 17.68 | 77.5 | 5.925 | 5.897 | 0.5 | 3.418 | 3.364 | 1.6 |
| $TaSe_2$ | 31.20 | 19.44 | 60.5 | 6.299 | 6.272 | 0.4 | 3.548 | 3.476 | 2.0 |
| $TiS_2$ | 29.21 | 18.88 | 54.7 | 5.685 | 5.705 | -0.4 | 3.440 | 3.409 | 0.9 |
| $TiSe_2$ | 29.13 | 17.39 | 67.5 | 6.032 | 6.004 | 0.5 | 3.589 | 3.536 | 1.5 |
| $TiTe_2$ | 31.04 | 19.76 | 57.1 | 6.597 | 6.498 | 1.5 | 3.835 | 3.777 | 1.5 |
| $VS_2$ | 32.51 | 25.61 | 26.9 | 5.830 | 5.755 | 1.3 | 3.225 | 3.221 | 0.1 |
| $VSe_2$ | 31.22 | 22.26 | 40.3 | 6.214 | 6.107 | 1.7 | 3.392 | 3.358 | 1.0 |
| $WS_2$ | 31.15 | 20.24 | 53.9 | 12.415 | 12.323 | 0.7 | 3.225 | 3.153 | 2.2 |
| $WSe_2$ | 30.34 | 19.98 | 51.9 | 13.159 | 12.960 | 1.5 | 3.367 | 3.282 | 2.6 |
| $ZrS_2$ | 24.91 | 16.98 | 46.7 | 5.810 | 5.813 | -0.1 | 3.710 | 3.662 | 1.3 |
| $ZrSe_2$ | 25.85 | 18.53 | 39.5 | 6.166 | 6.128 | 0.6 | 3.832 | 3.770 | 1.7 |
| $ZrTe_2$ | 30.3 | 16.34 | 85.4 | 6.735 | 6.660 | 1.2 | 4.020 | 3.952 | 1.7 |
| Graphite | 27.0 | 18.32 | 47.6 | 6.684 | 6.696 | -0.2 | 2.472 | 2.456 | 0.6 |
| MRE | | | 52.5 | | | 0.7 | | | 1.1 |
| MARE | | | 52.5 | | | 1.8 | | | 1.8 |

Table 5: PW86R-VV10sol binding energies and relaxed geometries for 26 weakly bonded layered compounds. Energies are given in meV/Å$^2$ and lattice constants in Å.

| Compound | $E_B$ | $E_B^{RPA}$ | RE [%] | $c$ | $c^{exp}$ | RE [%] | $a$ | $a^{exp}$ | RE [%] |
|---|---|---|---|---|---|---|---|---|---|
| BN | 15.77 | 14.49 | 8.8 | 6.874 | 6.690 | 2.7 | 2.516 | 2.510 | 0.2 |
| $HfS_2$ | 15.98 | 16.13 | -0.9 | 5.972 | 5.837 | 2.3 | 3.687 | 3.635 | 1.4 |
| $HfSe_2$ | 16.58 | 17.09 | -2.9 | 6.334 | 6.159 | 2.8 | 3.821 | 3.748 | 1.9 |
| $HfTe_2$ | 18.57 | 18.68 | -0.5 | 6.921 | 6.650 | 4.0 | 4.037 | 3.957 | 2.0 |
| $MoS_2$ | 20.26 | 20.53 | -1.2 | 12.625 | 12.302 | 2.6 | 3.241 | 3.162 | 2.4 |
| $MoSe_2$ | 19.69 | 19.63 | 0.3 | 13.365 | 12.927 | 3.3 | 3.387 | 3.289 | 2.9 |
| $MoTe_2$ | 20.21 | 20.80 | -2.8 | 14.531 | 13.973 | 3.9 | 3.626 | 3.518 | 3.0 |
| $NbSe_2$ | 22.01 | 19.57 | 12.4 | 12.928 | 12.547 | 3.0 | 3.542 | 3.442 | 2.8 |
| $NbTe_2$ | 23.91 | 23.03 | 3.8 | 7.036 | 6.610 | 6.4 | 3.775 | 3.680 | 2.5 |
| PbO | 18.64 | 20.25 | -7.9 | 5.167 | 4.995 | 3.4 | 4.105 | 3.964 | 3.5 |
| $PdTe_2$ | 31.40 | 40.17 | -21.8 | 5.328 | 5.113 | 4.2 | 4.170 | 4.024 | 3.6 |
| $PtS_2$ | 19.71 | 20.55 | -4.0 | 5.215 | 5.043 | 3.4 | 3.642 | 3.542 | 2.8 |
| $PtSe_2$ | 18.94 | 19.05 | -0.5 | 5.291 | 5.081 | 4.1 | 3.852 | 3.727 | 3.3 |
| $TaS_2$ | 20.63 | 17.68 | 16.6 | 6.082 | 5.897 | 3.1 | 3.432 | 3.364 | 1.9 |
| $TaSe_2$ | 20.73 | 19.44 | 6.6 | 6.450 | 6.272 | 2.8 | 3.562 | 3.476 | 2.4 |
| $TiS_2$ | 19.05 | 18.88 | 0.9 | 5.833 | 5.705 | 2.2 | 3.456 | 3.409 | 1.3 |
| $TiSe_2$ | 18.91 | 17.39 | 8.7 | 6.191 | 6.004 | 3.1 | 3.604 | 3.536 | 1.9 |
| $TiTe_2$ | 20.69 | 19.76 | 4.7 | 6.722 | 6.498 | 3.4 | 3.856 | 3.777 | 2.1 |
| $VS_2$ | 21.28 | 25.61 | -16.8 | 5.959 | 5.755 | 3.5 | 3.244 | 3.221 | 0.7 |
| $VSe_2$ | 20.67 | 22.26 | -7.1 | 6.370 | 6.107 | 4.3 | 3.404 | 3.358 | 1.3 |
| $WS_2$ | 20.54 | 20.24 | 1.4 | 12.712 | 12.323 | 3.1 | 3.237 | 3.153 | 2.6 |
| $WSe_2$ | 19.95 | 19.98 | -0.1 | 13.456 | 12.960 | 3.8 | 3.381 | 3.282 | 3.0 |
| $ZrS_2$ | 16.12 | 16.98 | -5.0 | 5.963 | 5.813 | 2.5 | 3.725 | 3.662 | 1.7 |
| $ZrSe_2$ | 17.06 | 18.53 | -7.9 | 6.308 | 6.128 | 2.9 | 3.853 | 3.770 | 2.2 |
| $ZrTe_2$ | 20.62 | 16.34 | 26.1 | 6.852 | 6.660 | 2.8 | 4.051 | 3.952 | 2.5 |
| Graphite | 16.52 | 18.32 | -9.8 | 6.983 | 6.696 | 4.2 | 2.473 | 2.456 | 0.7 |
| MRE | | | 0.04 | | | 3.4 | | | 2.2 |
| MARE | | | 6.9 | | | 3.4 | | | 2.2 |

Table 6: AM05-VV10sol binding energies and relaxed geometries for 26 weakly bonded layered compounds. Energies are given in meV/Å$^2$ and lattice constants in Å.

| Compound | $E_B$ | $E_B^{RPA}$ | RE [%] | $c$ | $c^{exp}$ | RE [%] | $a$ | $a^{exp}$ | RE [%] |
|---|---|---|---|---|---|---|---|---|---|
| BN | 15.15 | 14.49 | 4.6 | 6.839 | 6.690 | 2.2 | 2.507 | 2.510 | -0.1 |
| $HfS_2$ | 14.52 | 16.13 | -9.9 | 5.955 | 5.837 | 2.0 | 3.585 | 3.635 | -1.3 |
| $HfSe_2$ | 15.02 | 17.09 | -12.1 | 6.203 | 6.159 | 0.7 | 3.689 | 3.748 | -1.5 |
| $HfTe_2$ | 18.92 | 18.68 | 1.3 | 6.584 | 6.650 | -0.9 | 3.851 | 3.957 | -2.6 |
| $MoS_2$ | 21.05 | 20.53 | 2.5 | 12.397 | 12.302 | 0.7 | 3.140 | 3.162 | -0.6 |
| $MoSe_2$ | 18.57 | 19.63 | -5.3 | 13.043 | 12.927 | 0.9 | 3.260 | 3.289 | -0.8 |
| $MoTe_2$ | 22.61 | 20.80 | 8.7 | 13.888 | 13.973 | -0.6 | 3.474 | 3.518 | -1.2 |
| $NbSe_2$ | 23.06 | 19.57 | 17.8 | 12.270 | 12.547 | -2.2 | 3.415 | 3.442 | -0.7 |
| $NbTe_2$ | 28.09 | 23.03 | 22.0 | 6.713 | 6.610 | 1.5 | 3.601 | 3.680 | -2.1 |
| PbO | 23.68 | 20.25 | 16.9 | 4.972 | 4.995 | -0.4 | 3.991 | 3.964 | 0.6 |
| $PdTe_2$ | 46.09 | 40.17 | 14.7 | 5.029 | 5.113 | -1.6 | 4.028 | 4.024 | 0.1 |
| $PtS_2$ | 19.96 | 20.55 | -2.8 | 4.691 | 5.043 | -6.9 | 3.573 | 3.542 | 0.8 |
| $PtSe_2$ | 23.44 | 19.05 | 23.0 | 4.820 | 5.081 | -5.1 | 3.754 | 3.727 | 0.7 |
| $TaS_2$ | 19.23 | 17.68 | 8.7 | 5.946 | 5.897 | 0.8 | 3.305 | 3.364 | -1.7 |
| $TaSe_2$ | 19.76 | 19.44 | 1.6 | 6.252 | 6.272 | -0.3 | 3.425 | 3.476 | -1.4 |
| $TiS_2$ | 19.38 | 18.88 | 2.6 | 5.677 | 5.705 | -0.4 | 3.338 | 3.409 | -2.0 |
| $TiSe_2$ | 20.01 | 17.39 | 15.1 | 5.913 | 6.004 | -1.5 | 3.465 | 3.536 | -2.0 |
| $TiTe_2$ | 24.91 | 19.76 | 26.0 | 6.378 | 6.498 | -1.8 | 3.685 | 3.777 | -2.4 |
| $VS_2$ | 21.90 | 25.61 | -14.4 | 5.774 | 5.755 | 0.3 | 3.119 | 3.221 | -3.1 |
| $VSe_2$ | 21.55 | 22.26 | -3.1 | 6.157 | 6.107 | 0.8 | 3.263 | 3.358 | -2.8 |
| $WS_2$ | 18.35 | 20.24 | -9.3 | 12.530 | 12.323 | 1.6 | 3.137 | 3.153 | -0.4 |
| $WSe_2$ | 18.62 | 19.98 | -6.7 | 13.101 | 12.960 | 1.0 | 3.261 | 3.282 | -0.6 |
| $ZrS_2$ | 16.74 | 16.98 | -1.4 | 5.867 | 5.813 | 0.9 | 3.627 | 3.662 | -0.9 |
| $ZrSe_2$ | 17.58 | 18.53 | -5.1 | 6.128 | 6.128 | 0.0 | 3.729 | 3.770 | -1.0 |
| $ZrTe_2$ | 23.78 | 16.34 | 45.5 | 6.554 | 6.660 | -1.5 | 3.848 | 3.952 | -2.6 |
| Graphite | 17.20 | 18.32 | -6.1 | 6.991 | 6.696 | 4.4 | 2.461 | 2.456 | 0.2 |
| MRE | | | 5.2 | | | -0.2 | | | -1.2 |
| MARE | | | 11.1 | | | 1.6 | | | 1.4 |

Table 7: PW86R-VV10 lattice constants for 23 solids.

| Compound | $a_{calc}$ [Å] | $a_{ref}$ [Å] | Error [Å] | RE [%] | ARE [%] |
|---|---|---|---|---|---|
| Cu | 3.652 | 3.595 | 0.0572 | 1.59 | 1.59 |
| Ag | 4.186 | 4.056 | 0.1297 | 3.20 | 3.20 |
| Pd | 3.994 | 3.875 | 0.1190 | 3.07 | 3.07 |
| Rh | 3.888 | 3.793 | 0.0946 | 2.49 | 2.49 |
| Li | 3.409 | 3.449 | -0.0402 | -1.17 | 1.17 |
| Na | 4.129 | 4.210 | -0.0812 | -1.93 | 1.93 |
| K | 5.138 | 5.212 | -0.0742 | -1.42 | 1.42 |
| Rb | 5.471 | 5.576 | -0.1045 | -1.87 | 1.87 |
| Cs | 5.855 | 6.039 | -0.1844 | -3.05 | 3.05 |
| Ca | 5.457 | 5.553 | -0.0961 | -1.73 | 1.73 |
| Sr | 5.934 | 6.045 | -0.1112 | -1.84 | 1.84 |
| Ba | 4.939 | 4.995 | -0.0557 | -1.12 | 1.12 |
| Al | 4.029 | 4.020 | 0.0093 | 0.23 | 0.23 |
| C | 3.585 | 3.543 | 0.0418 | 1.18 | 1.18 |
| Si | 5.484 | 5.416 | 0.0680 | 1.26 | 1.26 |
| SiC | 4.396 | 4.342 | 0.0537 | 1.24 | 1.24 |
| Ge | 5.807 | 5.640 | 0.1666 | 2.95 | 2.95 |
| GaAs | 5.793 | 5.638 | 0.1549 | 2.75 | 2.75 |
| LiF | 4.031 | 3.964 | 0.0665 | 1.68 | 1.68 |
| LiCl | 5.103 | 5.056 | 0.0474 | 0.94 | 0.94 |
| NaF | 4.632 | 4.579 | 0.0527 | 1.15 | 1.15 |
| NaCl | 5.598 | 5.565 | 0.0326 | 0.59 | 0.59 |
| MgO | 4.255 | 4.184 | 0.0709 | 1.69 | 1.69 |
| Average | | | | 0.51 | 1.75 |

Table 8: PW86R-VV10sol lattice constants for 23 solids.

| Compound | $a_{calc}$ [Å] | $a_{ref}$ [Å] | Error [Å] | RE [%] | ARE [%] |
|---|---|---|---|---|---|
| Cu | 3.671 | 3.595 | 0.0755 | 2.10 | 2.10 |
| Ag | 4.216 | 4.056 | 0.1602 | 3.95 | 3.95 |
| Pd | 4.015 | 3.875 | 0.1401 | 3.62 | 3.62 |
| Rh | 3.902 | 3.793 | 0.1092 | 2.88 | 2.88 |
| Li | 3.413 | 3.449 | -0.0355 | -1.03 | 1.03 |
| Na | 4.146 | 4.210 | -0.0640 | -1.52 | 1.52 |
| K | 5.181 | 5.212 | -0.0314 | -0.60 | 0.60 |
| Rb | 5.532 | 5.576 | -0.0442 | -0.79 | 0.79 |
| Cs | 5.951 | 6.039 | -0.0880 | -1.46 | 1.46 |
| Ca | 5.481 | 5.553 | -0.0724 | -1.30 | 1.30 |
| Sr | 5.971 | 6.045 | -0.0737 | -1.22 | 1.22 |
| Ba | 4.987 | 4.995 | -0.0080 | -0.16 | 0.16 |
| Al | 4.035 | 4.020 | 0.0154 | 0.38 | 0.38 |
| C | 3.588 | 3.543 | 0.0451 | 1.27 | 1.27 |
| Si | 5.495 | 5.416 | 0.0795 | 1.47 | 1.47 |
| SiC | 4.401 | 4.342 | 0.0592 | 1.36 | 1.36 |
| Ge | 5.835 | 5.640 | 0.1948 | 3.45 | 3.45 |
| GaAs | 5.817 | 5.638 | 0.1795 | 3.18 | 3.18 |
| LiF | 4.050 | 3.964 | 0.0865 | 2.18 | 2.18 |
| LiCl | 5.139 | 5.056 | 0.0832 | 1.65 | 1.65 |
| NaF | 4.660 | 4.579 | 0.0812 | 1.77 | 1.77 |
| NaCl | 5.643 | 5.565 | 0.0779 | 1.40 | 1.40 |
| MgO | 4.267 | 4.184 | 0.0825 | 1.97 | 1.97 |
| Average | | | | 1.07 | 1.77 |

Table 9: AM05-VV10sol lattice constants for 23 solids.

| Compound | $a_{calc}$ [Å] | $a_{ref}$ [Å] | Error [Å] | RE [%] | ARE [%] |
|---|---|---|---|---|---|
| Cu | 3.551 | 3.595 | -0.0436 | -1.21 | 1.21 |
| Ag | 4.047 | 4.056 | -0.0089 | -0.22 | 0.22 |
| Pd | 3.872 | 3.875 | -0.0030 | -0.08 | 0.08 |
| Rh | 3.783 | 3.793 | -0.0105 | -0.28 | 0.28 |
| Li | 3.464 | 3.449 | 0.0148 | 0.43 | 0.43 |
| Na | 4.174 | 4.210 | -0.0359 | -0.85 | 0.85 |
| K | 5.228 | 5.212 | 0.0159 | 0.31 | 0.31 |
| Rb | 5.584 | 5.576 | 0.0080 | 0.14 | 0.14 |
| Cs | 6.033 | 6.039 | -0.0065 | -0.11 | 0.11 |
| Ca | 5.461 | 5.553 | -0.0923 | -1.66 | 1.66 |
| Sr | 5.930 | 6.045 | -0.1154 | -1.91 | 1.91 |
| Ba | 4.910 | 4.995 | -0.0851 | -1.70 | 1.70 |
| Al | 4.002 | 4.020 | -0.0181 | -0.45 | 0.45 |
| C | 3.552 | 3.543 | 0.0087 | 0.25 | 0.25 |
| Si | 5.428 | 5.416 | 0.0125 | 0.23 | 0.23 |
| SiC | 4.352 | 4.342 | 0.0104 | 0.24 | 0.24 |
| Ge | 5.652 | 5.640 | 0.0117 | 0.21 | 0.21 |
| GaAs | 5.651 | 5.638 | 0.0127 | 0.23 | 0.23 |
| LiF | 4.028 | 3.964 | 0.0644 | 1.63 | 1.63 |
| LiCl | 5.092 | 5.056 | 0.0361 | 0.71 | 0.71 |
| NaF | 4.643 | 4.579 | 0.0642 | 1.40 | 1.40 |
| NaCl | 5.626 | 5.565 | 0.0607 | 1.09 | 1.09 |
| MgO | 4.216 | 4.184 | 0.0319 | 0.76 | 0.76 |
| Average | | | | -0.03 | 0.70 |

Table 10: PW86R-VV10 interaction energies of the S22 training set.

| Complex | $E_{int}$ [eV] | $E_{ref}$ [eV] | error | RE [%] |
|---|---|---|---|---|
| | | H-bonded complexes | | |
| $(NH_3)_2$ | -0.15004 | -0.13669 | 0.01335 | 9.77 |
| $(H_2O)_2$ | -0.24900 | -0.21697 | 0.03203 | 14.7 |
| Formic acid dimer | -0.89010 | -0.81362 | 0.07647 | 9.39 |
| Formamide dimer | -0.73405 | -0.69689 | 0.03716 | 5.33 |
| Uracil dimer, HB | -0.89147 | -0.89563 | -0.00417 | -0.46 |
| 2-pyridoxine·2-aminopyridine | -0.79698 | -0.73508 | 0.06190 | 8.42 |
| Adenine·thymine, WC | -0.74088 | -0.72640 | 0.01448 | 1.99 |
| | | Dispersion dominated complexes | | |
| $(CH_4)_2$ | -0.02195 | -0.02300 | -0.00105 | -4.54 |
| $(C_2H_4)_2$ | -0.06375 | -0.06422 | -0.00047 | -0.73 |
| Benzene·$CH_4$ | -0.06165 | -0.06292 | -0.00127 | -2.02 |
| Benzene dimer, PD | -0.12247 | -0.11543 | 0.00704 | 6.10 |
| Pyrazine dimer | -0.18214 | -0.18485 | -0.00271 | -1.46 |
| Uracil dimer, stacked | -0.44320 | -0.42438 | 0.01882 | 4.43 |
| Indole·benzene, stacked | -0.20081 | -0.19614 | 0.00467 | 2.38 |
| Adenine·thymine stacked | -0.49756 | -0.50596 | -0.00841 | -1.66 |
| | | Mixed complexes | | |
| Ethene·ethine | -0.07310 | -0.06509 | 0.00801 | 12.3 |
| Benzene·$H_2O$ | -0.14303 | -0.14233 | 0.00070 | 0.48 |
| Benzene·$NH_3$ | -0.09643 | -0.10067 | -0.00424 | -4.20 |
| Benzene·HCN | -0.18766 | -0.19700 | -0.00934 | -4.74 |
| T-shaped benzene dimer | -0.11489 | -0.11803 | -0.00314 | -2.65 |
| T-shaped indole benzene | -0.23730 | -0.244330 | -0.00701 | -2.86 |
| Phenole dimer | -0.32787 | -0.30809 | 0.01978 | 6.41 |
| ME | | | | 2.6 |
| MAE | | | | 4.9 |

Table 11: PW86R-VV10sol interaction energies of the S22 training set.

| Complex | $E_{int}$ [eV] | $E_{ref}$ [eV] | error | RE [%] |
|---|---|---|---|---|
| H-bonded complexes | | | | |
| $(NH_3)_2$ | -0.13467 | -0.13669 | -0.00201 | -1.47 |
| $(H_2O)_2$ | -0.23469 | -0.21697 | 0.01773 | 8.17 |
| Formic acid dimer | -0.84054 | -0.81362 | 0.02692 | 3.31 |
| Formamide dimer | -0.68851 | -0.69689 | -0.00839 | -1.20 |
| Uracil dimer, HB | -0.83365 | -0.89563 | -0.06199 | -6.92 |
| 2-pyridoxine·2-aminopyridine | -0.73636 | -0.73508 | 0.00128 | 0.17 |
| Adenine·thymine, WC | -0.67198 | -0.72640 | -0.05442 | -7.49 |
| Dispersion dominated complexes | | | | |
| $(CH_4)_2$ | -0.01123 | -0.02300 | -0.01177 | -51.2 |
| $(C_2H_4)_2$ | -0.03861 | -0.06422 | -0.02561 | -39.9 |
| Benzene·$CH_4$ | -0.03256 | -0.06292 | -0.03037 | -48.3 |
| Benzene dimer, PD | -0.03544 | -0.11543 | -0.07998 | -69.3 |
| Pyrazine dimer | -0.09063 | -0.18485 | -0.09423 | -51.0 |
| Uracil dimer, stacked | -0.31170 | -0.42438 | -0.11268 | -26.6 |
| Indole·benzene, stacked | -0.07326 | -0.19614 | -0.12287 | -62.6 |
| Adenine·thymine stacked | -0.30824 | -0.50596 | -0.19772 | -39.1 |
| Mixed complexes | | | | |
| Ethene·ethine | -0.06102 | -0.06509 | -0.00407 | -6.26 |
| Benzene·$H_2O$ | -0.11390 | -0.14233 | -0.02843 | -20.0 |
| Benzene·$NH_3$ | -0.06731 | -0.10067 | -0.03337 | -33.1 |
| Benzene·HCN | -0.15250 | -0.19700 | -0.04451 | -22.6 |
| T-shaped benzene dimer | –0.06744 | -0.11803 | -0.05059 | -42.9 |
| T-shaped indole benzene | -0.17188 | -0.24430 | -0.07243 | -29.6 |
| Phenole dimer | -0.26932 | -0.30809 | -0.03877 | -12.6 |
| ME | | | | -25.5 |
| MAE | | | | 26.5 |

Table 12: AM05-VV10sol interaction energies of the S22 training set.

| Complex | $E_{int}$ [eV] | $E_{ref}$ [eV] | error | RE [%] |
|---|---|---|---|---|
| H-bonded complexes | | | | |
| $(NH_3)_2$ | -0.12116 | -0.13669 | -0.01553 | -11.4 |
| $(H_2O)_2$ | -0.22730 | -0.21697 | 0.01033 | 4.76 |
| Formic acid dimer | -0.89858 | -0.81362 | 0.08496 | 10.4 |
| Formamide dimer | -0.70802 | -0.69689 | 0.01113 | 1.60 |
| Uracil dimer, HB | -0.88166 | -0.89563 | -0.01397 | -1.56 |
| 2-pyridoxine·2-aminopyridine | -0.78352 | -0.73508 | 0.04844 | 6.59 |
| Adenine·thymine, WC | -0.71614 | -0.72640 | -0.01026 | -1.41 |
| Dispersion dominated complexes | | | | |
| $(CH_4)_2$ | 0.00109 | -0.02300 | -0.02409 | -104.7 |
| $(C_2H_4)_2$ | -0.01596 | -0.06422 | -0.04826 | -75.1 |
| Benzene·$CH_4$ | -0.01806 | -0.06292 | -0.04486 | -71.3 |
| Benzene dimer, PD | -0.01238 | -0.11543 | -0.10305 | -89.3 |
| Pyrazine dimer | -0.06785 | -0.18485 | -0.11700 | -63.3 |
| Uracil dimer, stacked | -0.27651 | -0.42438 | -0.14788 | -34.8 |
| Indole·benzene, stacked | -0.04231 | -0.19614 | -0.15383 | -78.4 |
| Adenine·thymine stacked | -0.26092 | -0.50596 | -0.24504 | -48.4 |
| Mixed complexes | | | | |
| Ethene·ethine | -0.05324 | -0.06509 | -0.01185 | -18.2 |
| Benzene·$H_2O$ | -0.10446 | -0.14233 | -0.03787 | -26.6 |
| Benzene·$NH_3$ | -0.05529 | -0.10067 | -0.04538 | -45.1 |
| Benzene·HCN | -0.15245 | -0.19700 | -0.04456 | -22.6 |
| T-shaped benzene dimer | -0.06810 | -0.11803 | -0.04993 | -42.3 |
| T-shaped indole benzene | -0.18209 | -0.24430 | -0.06221 | -25.5 |
| Phenole dimer | -0.26115 | -0.30809 | -0.04694 | -15.2 |
| ME | | | | -34.2 |
| MAE | | | | 36.3 |
